# Supplementary material for: Delocalization of Quasiparticle Moir\'e States in Twisted Bilayer hBN
Source: arXiv:2406.19700 ancillary file (2024-06-28)
Supplement: Supplementary file 1 [file SI.pdf]

# Supporting information for: Delocalization of Quasiparticle Moiré States in Twisted Bilayer hBN

Arsineh Apelian,[†] Annabelle Canestraight,[‡] Songyuan Liu,[¶] and Vojtěch Vlček[*,§,†]

†*Materials Department, University of California, Santa Barbara, CA 93106-9510, U.S.A.*

‡*Department of Chemical Engineering, University of California, Santa Barbara, CA 93106-9510, U.S.A.*

¶*Department of Physics, University of California, Santa Barbara, CA 93106-9510, U.S.A.*

§*Department of Chemistry and Biochemistry, University of California, Santa Barbara, CA 93106-9510, U.S.A.*

E-mail: vlcek@ucsb.edu

**DFT Computational Details** All *ab initio* relaxations and convergence tests are performed using a hexagonal unit cell in the Quantum ESPRESSO (QE)[1] code with Van der Waals interactions treated by the Tkatchenko-Scheffler total energy corrections.[2] We use a converged $6 \times 6 \times 1$ k-point grid with a kinetic energy cut-off of 30 Ha until energies are converged to $< 0.0025$ Ha. We use an in-plane lattice parameter of 2.498 Å and an optimized interlayer distance of 3.33 Å for all structures. The self-consistent DFT calculations are performed in a real-space implementation using rectangular/conventional cells, employing regular grids with $0.4 \times 0.4 \times 0.4$ grid spacing for $\theta = 5.09°$, $3.48°$, $2.88°$ and $0.43 \times 0.48 \times 0.45$ grid spacing for $\theta = 2.45°$. Troullier-Martins pseudopotentials[3] and the

PBE[4] functional for exchange and correlation are employed. We use a kinetic energy cut-off of 30 Ha and a vacuum layer of 24 Å to cut off periodic images along the $z$ direction. Also, to ensure 2D periodicity of the bilayer, we use modified periodic boundary conditions with Coulomb interaction cutoffs.[5] Overall, the Kohn-Sham eigenvalues are converged to $< 10$ meV.

Three high-symmetry points (AA, AB, SP) are identified as shown in Fig.1 (a) of the main text. In the AA stacking arrangement, the hexagonal rings sit on top of each other with B and N atoms directly aligned along the c-axis, for the AB stacking arrangement, the bottom layer of atoms is shifted by one bond length ($\approx 1.4$ Å) along the b-axis, and lastly, for the saddle-point stacking arrangement (SP), the bottom layer of atoms are shifted by the same amount along the c-axis. The individual high-symmetry regions (AA, AB, SP) band gaps are converged with respect to simulation cell sizes: $(7 \times 4)$, $(14 \times 8)$, and $(21 \times 12)$.

**Stochastic many-body theory** Here, we employ the many-body perturbation theory and use DFT eigenvalues and orbitals ($\epsilon_j^{DFT}$ and $\phi_j$) as a starting point calculation for obtaining the QP energies. An energy correction is added, which represents the difference between the exchange-correlation ($\hat{v}_{xc}$) potential (already included in the KS Hamiltonian of DFT) and the xc self-energy ($\hat{\Sigma}_{xc}$) which is the non-local and dynamical many-body interactions potential. The self-energy is constructed using the $GW$ approximation, which combines electron exchange interaction with dynamical screening due to the charge density oscillations, written as $\Sigma_{xc}^{GW}(\mathbf{r},\mathbf{r}',t) = iG(\mathbf{r},\mathbf{r}',t)W(\mathbf{r},\mathbf{r}',t)$, where $G$ is the Green's function (a QP propagator) which describes the probability amplitude for a hole to propagate from one space-time $(\mathbf{r},t)$ to another $(\mathbf{r}',t')$. The Green's function can be written in the Lehmann representation as:

$$G(\mathbf{r}',r,\omega) = \sum_j \frac{\Psi_j^{N-1}(\mathbf{r})\Psi_j^{N-1^*}(\mathbf{r})}{\hbar\omega - \epsilon_j^{N-1} + i\eta} \qquad (1)$$

where the Dyson orbitals are obtained as $\Psi_n(\mathbf{r}) = \langle \Psi_{N-1}^n | \hat{\Psi}(\mathbf{r}) | \Psi_N^0 \rangle$ from the $N$-particle ground state and the $n$-th excited state of the $(N-1)$ particle system, where the $\hat{\Psi}(\mathbf{r})$ is

the field operator, and $n$ runs over all hole (occupied) states in the system. The Green's function has poles at the many-particle excitation energy $\epsilon_j^{N-1}$ associated with the hole states. Charge addition, i.e. electron propagation from $(\mathbf{r}', t')$ to $(\mathbf{r}, t)$ is treated analogously for the $(N+1)$ particle system. Finally, $W$ is the screened Coulomb interaction: $W(\mathbf{r}, \mathbf{r}', t) = \int \epsilon^{-1}(\mathbf{r}, \mathbf{r}_1, t)\nu(\mathbf{r}_1, \mathbf{r}', t)d\mathbf{r}_1$ where $\epsilon^{-1}$ is the inverse dielectric function. Calculations are typically not performed self-consistently, and so the QP energies are obtained by a "one-shot" correction, conventionally denoted as $G_0W_0$. Specifically, for the $j$th KS eigenstate, the QP energies are obtained as: $\epsilon_j = \epsilon_j^{DFT} + \langle\phi_j|\hat{\Sigma}_{xc}(\epsilon_j) - \hat{v}_{xc}|\phi_j\rangle$ where the self-energy is evaluated at the QP energy itself, i.e. it is evaluated as a fixed-point solution at the frequency corresponding to the QP energy. In this case, $\{\phi_j\}$ represents the single-particle states from the mean-field DFT calculation, i.e. the KS basis is not updated and the Dyson orbitals are not computed at the $G_0W_0$ level, in which merely a self-energy correction is added to the single-particle energies. To go beyond this approximation, the QP Hamiltonian matrix must be fully diagonalized, yielding the Dyson orbitals.

Quantitative understanding of QPs in twisted bilayers is limited by the large system sizes that need to be considered, therefore, conventional $GW$ cannot treat these systems.[6] Here, we overcome these limitations by implementing the linear-scaling stochastic real-time $GW$ method, which is a statistical approach in which the expectation values of the self-energy are sampled using random vectors in the Hilbert space.[7–9] In practice, we first separate the exchange part $\Sigma_X$ and the correlation self-energy, $\Sigma_c(t)$, is computed stochastically in the time domain in two steps: (i) the Green's function is sampled using random vectors within the occupied/unoccupied subspace (describing holes/electron), propagated backward/forward in time to comply with the the time ordering and (ii) the action of the screened Coulomb interaction is sampled via random vectors representing the induced charge density oscillation. Lastly, to obtain the Dyson orbitals, we truncate the full Hamiltonian matrix onto a stochastic basis and construct random vectors which are mutually orthogonalized. Since orthogonalization is a unitary transformation, this does not impact the resulting eigenstates.

The full frequency diagonalization of the QP Hamiltonian is described in[10] and it is employed for the compressed representation as detailed in the main text.

**s-$G_0W_0$ and gap variation** The $G_0W_0$ calculations were performed using the Stochastic$GW$ code.[7–9] The sampling of the Green's function $G$ was performed using $N_\zeta = 400$ random vectors. $N_\eta = 16$ was used to sample the induced charge density in the real time-time RPA calculation (in the $W$ part of $GW$). The final stochastic error on the quasiparticle energies is $\leq 25$ meV. Full results for each twist angle and region using DFT and s-$G_0W_0$ are shown in Table 1. All s-$G_0W_0$ band gap values have a statistical error of 0.04 eV or less.

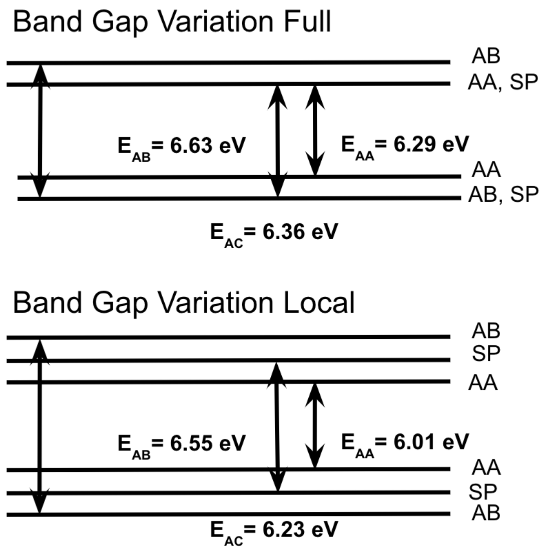


Table S.1: Band gaps (eV) for each region

| $\theta$ | Region | DFT | s-$G_0W_0$ |
|---|---|---|---|
| 0° | AA | 3.86 | 6.01 |
| | AB | 4.51 | 6.55 |
| | SP | 4.14 | 6.23 |
| 2.45° | AA | 4.01 | 6.22 |
| | AB | 4.47 | 6.61 |
| | SP | 4.18 | 6.24 |
| 2.88° | AA | 4.06 | 6.19 |
| | AB | 4.48 | 6.63 |
| | SP | 4.22 | 6.30 |
| 3.48° | AA | 4.09 | 6.21 |
| | AB | 4.54 | 6.69 |
| | SP | 4.27 | 6.32 |
| 5.09° | AA | 4.16 | 6.29 |
| | AB | 4.44 | 6.63 |
| | SP | 4.26 | 6.36 |

Figure S.1: Band gap variation shown using s-$G_0W_0$ according to the full, twisted structures (top) vs local environment (bottom) for $\theta = 5.09°$ by looking at LDOS plots and associated QP energies. Similarly, we do this procedure for all twist angles where the results are shown in Table S.1

**Moiré Potential Fit** We employ a second-order harmonic expansion, given by eq. (1) in the main text, to account for the SP regions (and AA-SP hybridized states) in the moiré potential. Fig. S.2 illustrates the line plots along $y = 0$ of the moiré potential fit against the s-$G_0W_0$ band gap data points for all twist angles. Table S.2 lists the fitting parameters for each moiré potential.

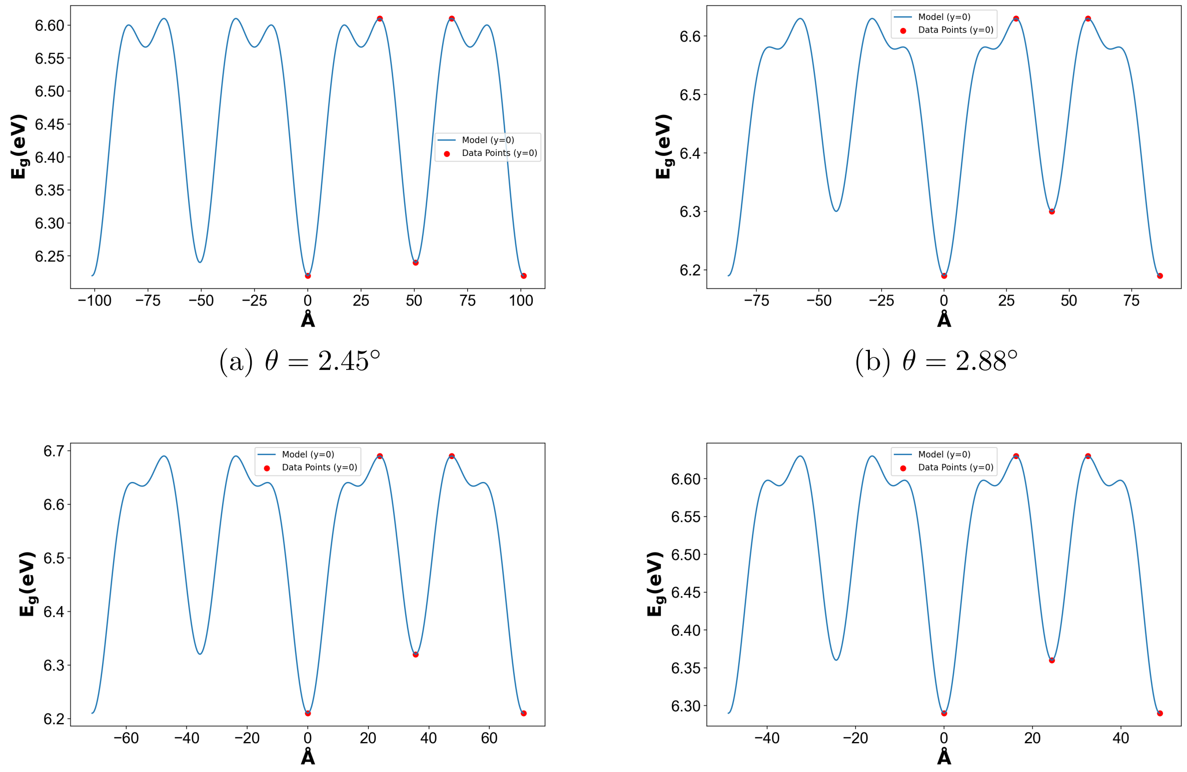


(a) $\theta = 2.45°$ (b) $\theta = 2.88°$

(c) $\theta = 3.48°$ (d) $\theta = 5.09°$

Figure S.2: Line plots (along $y = 0$) showing the moiré potential fit (blue lines) according to Eq. 1 (in main text) and data points (red dot) for $\theta =$ (a) 2.45° (b) 2.88° (c) 3.48° and (d) 5.09°

Table S.2: Moiré Potential Fitting Parameters

| $\theta$ | $V_0$ (eV) | $V_1$ (eV) | $V_2$ (eV) |
|---|---|---|---|
| 2.45° | 6.48 | -0.0050 | -0.0817 |
| 2.88° | 6.48 | -0.0275 | -0.0703 |
| 3.48° | 6.53 | -0.0275 | -0.0792 |
| 5.09° | 6.52 | -0.0175 | -0.0581 |

## Local Density of States (LDOS)

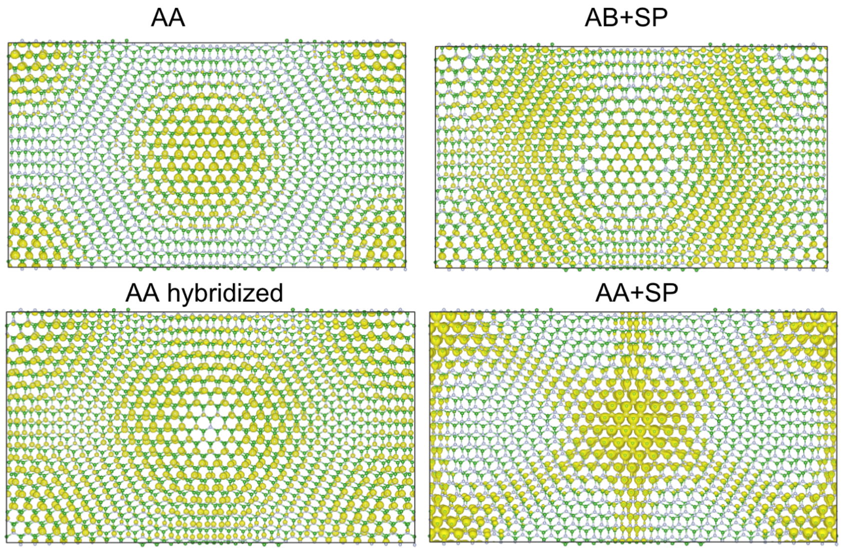


Figure S.3: LDOS for $\theta = 3.48°$ which shows AA, AA hybridized, and AB+SP localization for the valence states and AA+SP localization for the conduction states. These identified states are used for the stochastic compression

## Average Self-energy

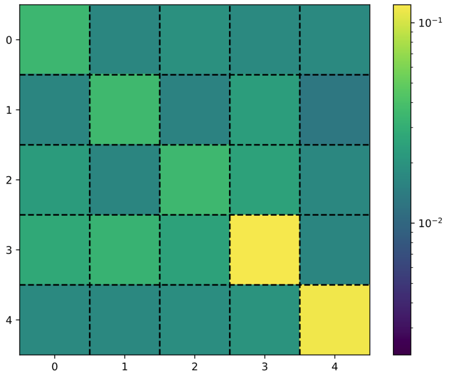


(a) Self-energy matrix for $\theta = 2.45°$

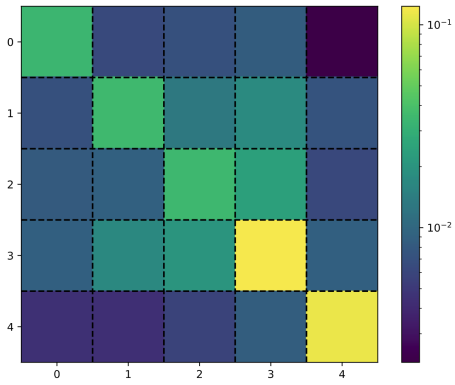


(b) Self-energy matrix for $\theta = 3.48°$

Figure S.4: Full Hamiltonian matrices for only the correlation self-energy, $\Sigma_c(t)$, compressed to a $5 \times 5$ matrix

# References


(1) Giannozzi, P.; Baseggio, O.; Bonfà, P.; Brunato, D.; Car, R.; Carnimeo, I.; Cavazzoni, C.; de Gironcoli, S.; Delugas, P.; Ferrari Ruffino, F.; Ferretti, A.; Marzari, N.; Timrov, I.; Urru, A.; Baroni, S. Quantum ESPRESSO toward the exascale. *The Journal of Chemical Physics* **2020**, *152*, 154105.

(2) Tkatchenko, A.; Scheffler, M. Accurate Molecular van der Waals Interactions from Ground-State Electron Density and Free-Atom Reference Data. *Phys. Rev. Lett.* **2009**, *102*, 073005.

(3) Troullier, N.; Martins, J. Efficient Pseudopotentials for Plane-Wave Calculations. *Phys. Rev. B* **1991**, *43*, 1993–2006.

(4) Perdew, J. P.; Wang, Y. Accurate and Simple Analytic Representation of the Electron-gas Correlation Energy. *Phys. Rev. B* **1992**, *45*, 13244–13249.

(5) Rozzi, C. A.; Varsano, D.; Marini, A.; Gross, E. K. U.; Rubio, A. Exact Coulomb Cutoff Technique For Supercell Calculations. *Phys. Rev. B* **2006**, *73*, 205119.

(6) Brooks, J.; Weng, G.; Taylor, S.; Vlček, V. Stochastic Many-Body Perturbation Theory for Moiré States in Twisted Bilayer Phosphorene. *J. Phys.: Condens. Matter* **2020**, *32*, 234001.

(7) Vlček, V.; Li, W.; Baer, R.; Rabani, E.; Neuhauser, D. Swift GW Beyond 10,000 Electrons Using Sparse Stochastic Compression. *Phys. Rev. B* **2018**, *98*, 075107.

(8) Vlček, V.; Rabani, E.; Neuhauser, D.; Baer, R. Stochastic GW Calculations for Molecules. *J. Chem. Theory Comput.* **2017**, *13*, 4997–5003.

(9) Neuhauser, D.; Gao, Y.; Arntsen, C.; Karshenas, C.; Rabani, E.; Baer, R. Breaking the Theoretical Scaling Limit for Predicting Quasiparticle Energies: The Stochastic *GW* Approach. *Phys. Rev. Lett.* **2014**, *113*, 076402.

(10) Canestraight, A.; Lei, X.; Ibrahim, K. Z.; Vlček, V. Efficient Quasiparticle Determination beyond the Diagonal Approximation via Random Compression. *Journal of Chemical Theory and Computation* **2024**, *20*, 551–557, PMID: 38175913.
